# Supplementary material for: Quasiperiodic acceleration of electrons by a plasmoid-driven shock in the solar atmosphere
Source: arXiv:1406.0743 source file (2014-06-03)
Supplement: Supplementary file 1 [file gallagher_supplemntary_final.pdf]

# Quasi-periodic acceleration of electrons by a plasmoid-driven shock in the solar atmosphere
## *Supplementary Material*

August 20, 2013

### Alfvén Speed in the Corona and Mach Number of Radio Source

The propagation speed of Alfvén waves in a plasma with unperturbed magnetic field $B$ and mass density $\rho$ is given by

$$v_A = \frac{B}{\sqrt{4\pi\rho}} \tag{1}$$

Given the radio source had a frequency of emission of 150 MHz, we first convert to density using equation (3) below, and assuming that the emission is harmonic, this results in a density of $n_e = 6.9 \times 10^7\,\mathrm{cm}^{-3}$. Six AIA passbands were then used to create emission measure and density maps of the corona from $1.0-1.3\,R_\odot$ [1]. From $2.0-4.0\,R_\odot$ density diagnostics were performed using the LASCO C2 coronagraph [2]. At each position angle around the Sun, a set of hydrostatic equilibrium (HE) models were fit to the density data from AIA and C2 to form a continuous density map from $1.0-4.0\,R_\odot$. The HE models had the form:

$$n(r) = n_{ar}\exp\left(-\frac{rm_pg}{kT}\right) + n_{qs}\exp\left[-\frac{\mu m_p GM_\odot}{kTR_\odot}\left(\frac{r_0}{r}-1\right)\right] \tag{2}$$

where $r$ is heliocentric distance, $m_p$ is a proton mass, $g$ is acceleration due to gravity, $T$ is temperature, $k$ is Boltzman's constant, $G$ is the universal gravitational constant, $M_\odot$ is the solar mass, and $R_\odot$ is the solar radius. Here, the plane parallel model for $n_{ar}$ corresponds to the active region of the data derived from the EUV images, while the second spherically symmetric model corresponds to the quiet corona ($n_{qs}$) C2 data. These density diagnostics allowed a determination of the height from which 75 MHz originated. We find that over the range of the position angles encountered by the radio source, this frequency occurs at an average height of $1.27\,R_\odot$, with a maximum height of $1.31\,R_\odot$ and a minimum height of $1.21\,R_\odot$. If we add to this the uncertainty in position due to uncertainty in the density measurements themselves (15%), the heliocentric distance of the source comes to $1.27^{+0.06}_{-0.09}\,R_\odot$. This position, including uncertainties, combined with the value for angular velocity from Figure 2 in the main Article ($6.2 \pm 0.1 \times 10^{-4}\,\mathrm{rad\,s^{-1}}$), gives the tangential velocity of $548^{+34}_{-48}\,\mathrm{km\,s^{-1}}$ for the radio source.

Calculation of the Alfvén speed required a value of the magnetic field at the average heliocentric distance of the source, derived from potential field source surface (PFSS) extrapolation of the photospheric field strength (Supplementary Figure 2). At the source heliocentric distance of $1.27\,R_\odot$ we find $B = 0.67\,\mathrm{G}$. Combining this with the density at the radio source results in an Alfvén speed of $225\,\mathrm{km\,s^{-1}}$. Taking into account that the source may be in the range from $1.18-1.33\,R_\odot$ we find a possible range of $0.5-0.9\,\mathrm{G}$ for the magnetic field that the source may encounter between the position angles of $100-135°$. Again using the density at the radio source we find the possible range in Alfvén speeds that the source may encounter is $190-310\,\mathrm{km\,s^{-1}}$. Hence we quote the Alfvén speed as $v_A = 225^{+85}_{-35}\,\mathrm{km\,s^{-1}}$. Using the speed of the source we then find the Alfvén Mach to be $M_A = 2.4^{+0.7}_{-0.8}$. We note that it is not possible to estimate an error on the magnetic field strength since it is an extrapolation from the surface field, however, the results of super-Alfvénic Mach are tolerant to within 50% uncertainty on the PFSS B-field estimate. Also, the PFSS represents the lowest energy state of the coronal magnetic field, hence this Mach number is taken to be an upper limit.

Finally, the direction of the field is also given by the PFSS extrapolation. It shows an extended region of open and radial field structure in the south east quadrant of the corona, with a weak closed field region on disk in this quadrant. The shock propagated transversely through this region, showing there is a strong possibility of the shock encountering quasi-perpendicular orientation of the magnetic field.

## Frequency Drift and Particle Speeds

From the dynamic spectra it is possible to obtain a set of frequency time measurements $(f_i, t_i)$, in this case along the left edge of the type III. Using the expression for plasma oscillation

$$f_p = \frac{1}{2\pi}\left(\frac{n_e e^2}{\epsilon_0 m_e}\right)^{\frac{1}{2}} \tag{3}$$

where $n_e$ is electron number density, $e$ is electron charge, $\epsilon_0$ permittivity of free space, $m_e$ electron mass. The set $(f_i, t_i)$ may be converted into a set of density time values $(n_i, t_i)$ using equation (3). In order to convert these into a height-time set $(r_i, t_i)$, a density model of the solar corona is used. The density model in this case is derived from a solution to the Parker solar wind equation which is used specifically to analyze low frequency (interplanetary) type IIIs [3]. Once this $(r_i, t_i)$ height-time set was found, we took into account that the electron beams are traveling along open magnetic field lines which follow the Parker spiral. In cylindrical coordinates, the radius $r$ and azimuthal angle $\phi$ share the relationship $r - r_0 = -\frac{v_{sw}}{\Omega_\odot}(\phi - \phi_0)$ i.e., an Archimedean spiral with parameters $v_{sw}$, the solar wind velocity, and $\Omega_\odot$, the angular velocity at solar equator. The arch-length along any arm of this spiral (along an open magnetic field line) is given by

$$s(\phi) = \frac{v_{sw}}{2\Omega_\odot}(\phi\sqrt{1+\phi^2} + \text{arcsinh}(\phi)) \tag{4}$$

where arcsinh is the inverse hyperbolic sine function. Using a solar wind velocity value of $450\,\text{km}\,\text{s}^{-1}$ (observed in-situ using the STEREO-B PLASTIC instrument), and $\phi = \frac{\Omega_\odot}{v_{sw}} r = -6.5 \times 10^{-12}\,\text{rad}\,\text{m}^{-1} \times r$, the set $(r_i, t_i)$

were converted to a set of distances along the Parker spiral vs time $(s_i, t_i)$. A linear fit to this data then gives the speed of electrons producing the type III. While it is difficult to estimate an error on this speed, due to a lack of interplanetary density measurements from which this speed is derived, we may confirm the presence of particles with such energy from in-situ data. Supplementary Figure 3 shows a plot of electron flux versus time from the SEPT instrument on STEREO-B. It shows an increase in electron flux in the range of 45 - 325 keV. The vertical black line is the expected time of arrival of the electrons causing the type III burst, calculated from their speed and distance travelled on the Parker spiral. The expected time of arrival of the type III electrons match quite well the first peak in flux of the in-situ detected electrons, showing that the speeds derived from frequency drift are a reliable estimate.

The distances travelled by the electrons producing the herringbone emission are much shorter than the type III emission (indicated by their much shorter length in frequency space). This much shorter travelled distance does not require a conversion from height-time $(r_i, t_i)$ to distances along a spiral $(s_i, t_i)$, so electron beam speed for the herringbones was derived from a linear fit to the $(r_i, t_i)$ values.

## Supplementary Movie 1

The propagation of 150 MHz source and coronal bright front (CBF). The panels on the left show the solar radio burst activity in the dynamic spectra. The white line indicates the current time of the image sequence. The right panel shows the Atmospheric Imaging Assembly (AIA) 21.1 nm (blue image) with a heliographic grid of 15° spacing overplotted. The contours are 150 MHz observations from the Nancay Radioheliograph (NRH). The contours change colour according to the brightness temperature, indicated by the colour bar on the left. Brightness temperatures of up to $10^9$ K indicate that this is coherent plasma emission, generated by the presence of high velocity electrons. Hence the radio source is a site of electron acceleration that follows the propagation of the CBF closely.

## Supplementary Movie 2

In order to investigate any thermal properties of the CBF we have produced a tri-colour running ratio movie, see Supplementary Movie 2. The filters and colours used are 17.1 (blue), 19.3 (green), and 21.1 (red) nm. As described in [4], an excess in any one or two of these colours in such a tri-colour movie may indicate a local temperature change due to a passing transient. For example, a positive temperature perturbation (heating) may show up as excess emission in 19.3 nm and/or 21.1 nm passbands resulting in a orange/yellow appearance. A negative temperature perturbation (cooling) will result in excess 17.1 nm channel combined with a deficiency in 19.3 nm and 21.1 nm channels: this results in a blue appearance in the image. In this way, we can identify what parts of the CBF are due to local heating and what parts are due to cooling. This tri-colour analysis is especially important for identifying any multi-component nature to the event i.e., studies have suggested that CBFs may have both wave and magnetic reconfiguration properties [4, 5, 6](a hybrid of the wave and non-wave theories of CBFs). Analysing the thermal properties via the tri-colour method can reveal the presence of wave-like thermal properties. The furthermost front has a yellow appearance, indicative of a positive temperature perturbation, with a secondary blue (cooler) front behind it. This is the expected behaviour of a propagating pressure pulse i.e., a traveling pressure perturbation will result in a slight heating followed by a rarefaction and cooling in its wake, this concept is discussed in detail by [4]. This is further confirmation that the CBF observed in this event is indeed a pressure pulse, making it more likely to be associated with shock activity higher in the corona.

## Supplementary Figures

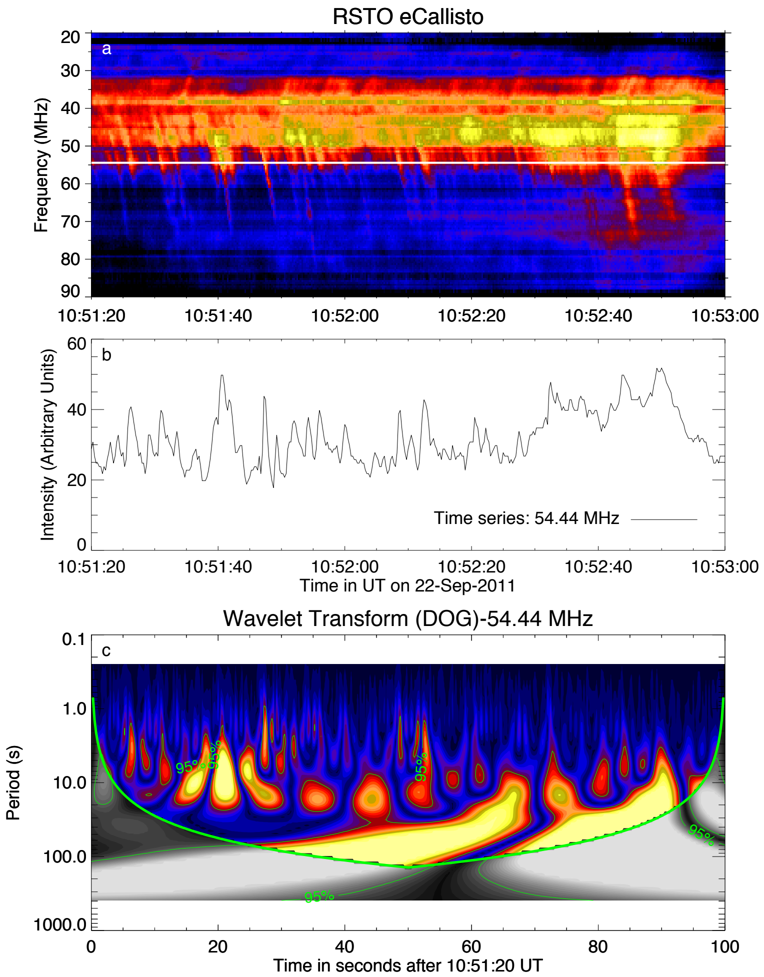


Figure 1: Wavelet analysis of herringbone radio bursts. Panel **a** shows the herringbones, the white line is the frequency from which a time-series has been extracted (54.44 MHz). Panel **b** shows the time series. Panel **c** shows a wavelet analysis of the time series using a derivative of a Gaussian (DOG) wavelet. The shaded grey area is the region outside the cone of influence and the green contours mark the 95% confidence level. The wavelet transform shows power in the regions of 2-11 seconds, revealing strong levels of periodicity throughout the time series.

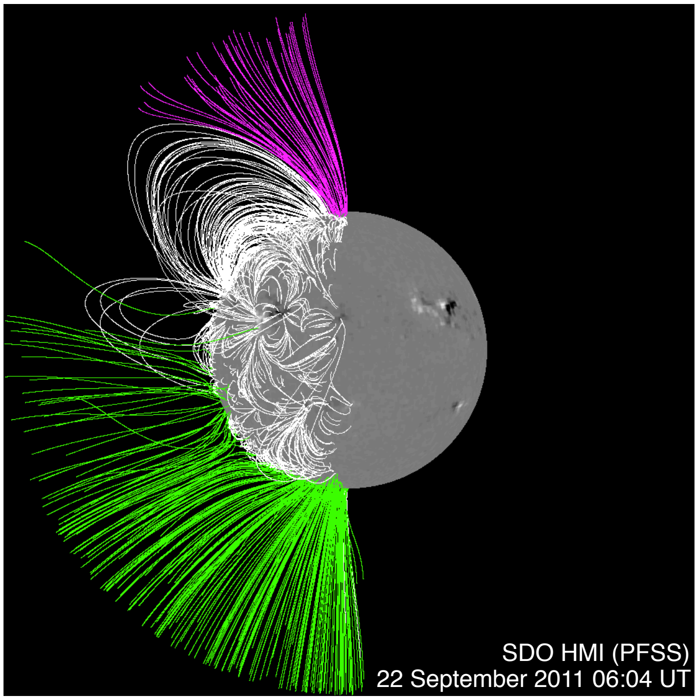


Figure 2: A potential field source surface (PFSS) extrapolation of the coronal magnetic field on the 22-Septemper-2011 06:04 UT. This was performed using the SolarSoft package of [7] and data from the Helioseismic and Magnetic Imager (HMI)[8] of the SDO spacecraft. Green and pink lines signify open field regions while white is closed field. The CBF and CME flank propagated through the south-east quadrant. Therefore a transverse propagation through these open and closed field structures suggests that the shock was likely of quasi-perpendicular orientation. Such a configuration is in agreement with the assertions of [9, 10], whereby a shock traveling parallel to the solar surface (as indicated by the transverse motion of the radio source in Figure 1 in the main Article) could produce herringbones with near-zero backbone drift. The type II followed by zero-drift herringbones may then indicate an initially radially driven shock, a component of which may then decouple and begin a transverse motion, thus producing the herringbones.

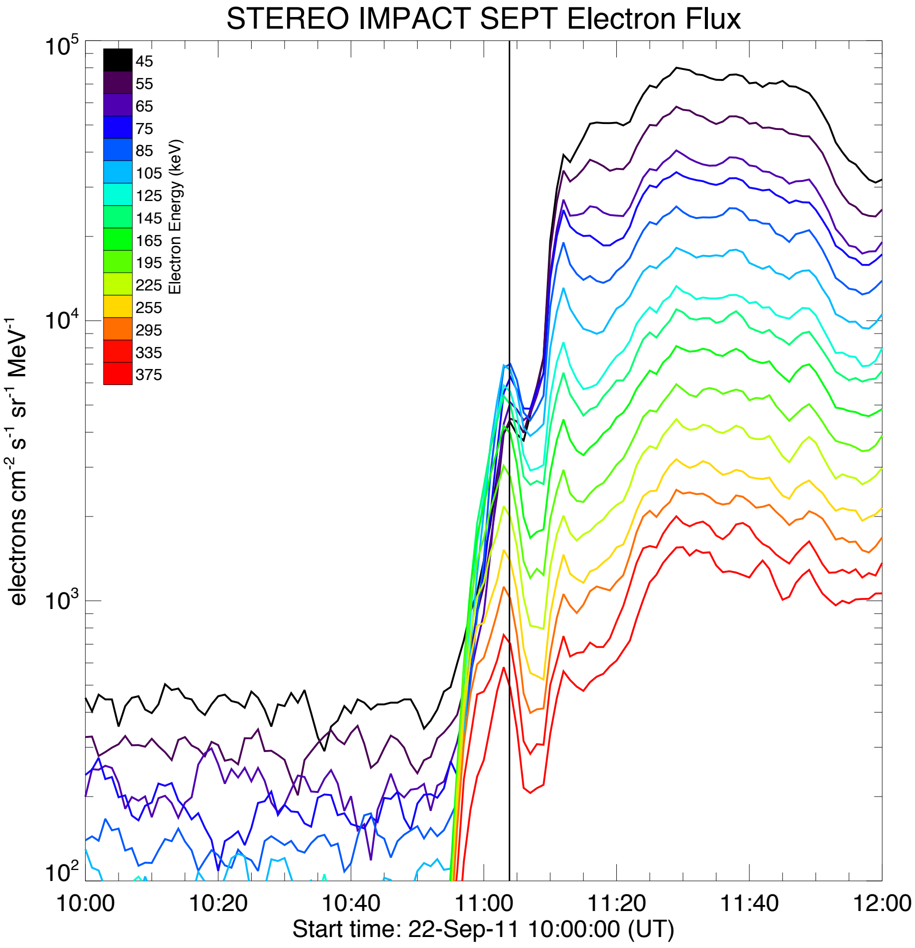


Figure 3: Detection of electrons in-situ by the Solar Electron Proton Telescope (SEPT)[11] instrument on board the STEREO-B spacecraft [12]. The electrons arrive at ∼11:05 UT, approximately 35 minutes after the flare start time. The black vertical line indicates the expected time of arrival (ETA) of the type III electrons. This ETA was calculated from the electron speed (derived from the frequency drift and a density model), and the distance travelled along the Parker spiral (given a solar wind speed of 450 $\mathrm{km\,s^{-1}}$). Note that the type III electrons, calculated to have an energy of 46 keV, have an ETA that is centered on the first peak in electron fluxes as detected by the SEPT low energy channels at 45 keV. This good agreement between predicted ETA and observed time of arrival, showing the type III electron energies are a sound estimate.

## References

[1] Aschwanden, M. J., Boerner, P., Schrijver, C. J. & Malanushenko, A. Automated Temperature and Emission Measure Analysis of Coronal Loops and Active Regions Observed with the Atmospheric Imaging Assembly on the Solar Dynamics Observatory (SDO/AIA). *Sol. Phys.* **283**, 5–30 (2013).

[2] van de Hulst, H. C. The electron density of the solar corona. *Bull. Astron. Inst. Netherlands* **11**, 135 (1950).

[3] Mann, G., Jansen, F., MacDowall, R. J., Kaiser, M. L. & Stone, R. G. A heliospheric density model and type III radio bursts. *A&A* **348**, 614–620 (1999).

[4] Downs, C., Roussev, I. I., van der Holst, B., Lugaz, N. & Sokolov, I. V. Understanding SDO/AIA Observations of the 2010 June 13 EUV Wave Event: Direct Insight from a Global Thermodynamic MHD Simulation. *ApJ* **750**, 134 (2012).

[5] Cohen, O., Attrill, G. D. R., Manchester, W. B., IV & Wills-Davey, M. J. Numerical Simulation of an EUV Coronal Wave Based on the 2009 February 13 CME Event Observed by STEREO. *ApJ* **705**, 587–602 (2009). 0909.3095.

[6] Cheng, X. *et al.* Investigation of the Formation and Separation of an Extreme-ultraviolet Wave from the Expansion of a Coronal Mass Ejection. *ApJ* **745**, L5 (2012). 1112.4540.

[7] Schrijver, C. J. & De Rosa, M. L. Photospheric and heliospheric magnetic fields. *Sol. Phys.* **212**, 165–200 (2003).

[8] Scherrer, P. H. *et al.* The Helioseismic and Magnetic Imager (HMI) Investigation for the Solar Dynamics Observatory (SDO). *Sol. Phys.* **275**, 207–227 (2012).

[9] Stewart, R. T. & Magun, A. Radio evidence for electron acceleration by transverse shock waves in herringbone Type II solar bursts. *Proceedings of the Astronomical Society of Australia* **4**, 53–55 (1980).

[10] Wild, J. P. Radio Observations of Solar Flares. *NASA Special Publication* **50**, 161 (1964).

[11] Müller-Mellin, R. *et al.* The Solar Electron and Proton Telescope for the STEREO Mission. *Space Sci. Rev.* **136**, 363–389 (2008).

[12] Kaiser, M. L. *et al.* The STEREO Mission: An Introduction. *Space Sci. Rev.* **136**, 5–16 (2008).
